# Supplementary material for: Physics-based Digital Twins for Autonomous Thermal Food Processing: Efficient, Non-intrusive Reduced-order Modeling
Source: arXiv:2209.03062 source file (2022-09-07)
Supplement: Supplementary file 1 [file Kannapinn2022_ROM_DigitalTwin_IFSET_SupplementaryMaterial.pdf]

# Physics-based Digital Twins for Autonomous Thermal Food Processing: Efficient, Non-intrusive Reduced-order Modeling

Maximilian Kannapinn<sup>a,b,\*</sup>, Minh Khang Pham<sup>c</sup>, Michael Schäfer<sup>a,b</sup>

<sup>a</sup>Institute for Numerical Methods in Mechanical Engineering, Technical University of Darmstadt, Dolivostr. 15, Darmstadt, 64293, Germany

<sup>b</sup>Graduate School Computational Engineering, Technical University of Darmstadt, Dolivostr. 15, Darmstadt, 64293, Germany

<sup>c</sup>Technical University of Darmstadt, Karolinenplatz 5, Darmstadt, 64289, Germany

---

## Abstract

Supplementary material

---

## 1. Correlations on test sets sinAP15 and MS15

Table 1: Correlations between error measures (rows) and a priori and a posteriori excitation signal KPIs (columns) for APRBS 1-signal-ROMs (test set: sinAP15).

|                | $\bar{T}_i$ | $\overline{T_{\text{diff},i}}$ | $\overline{T_{\text{diff},j}}$ | $ \overline{T_{\text{diff},i}} $ | $\bar{T}_{\text{oven}}$ | $\text{STD}(T_{\text{oven}})$ | $\text{Cr}(T_{\text{oven}})$ | $\text{Cv}(T_{\text{oven}})$ | $\text{Cv}(T_B)$ | $\text{Cv}(T_{\text{oven}}, T_B)$ | $\text{STD}(T_A)$ | $\text{STD}(T_B)$ |
|----------------|-------------|--------------------------------|--------------------------------|----------------------------------|-------------------------|-------------------------------|------------------------------|------------------------------|------------------|-----------------------------------|-------------------|-------------------|
| RMSE           | 0.10        | -0.45                          | -0.68                          | 0.28                             | 0.22                    | -0.14                         | -0.11                        | 0.26                         | -0.37            | 0.19                              | 0.01              | -0.72             |
| MAPE           | 0.16        | -0.43                          | -0.69                          | 0.34                             | 0.29                    | -0.13                         | -0.12                        | 0.26                         | -0.32            | 0.26                              | 0.00              | -0.74             |
| MAX            | -0.04       | -0.52                          | -0.64                          | 0.15                             | 0.04                    | -0.17                         | -0.07                        | 0.24                         | -0.47            | 0.01                              | 0.05              | -0.64             |
| MEDIAN         | 0.18        | -0.43                          | -0.75                          | 0.48                             | 0.34                    | -0.08                         | -0.13                        | 0.19                         | -0.35            | 0.39                              | -0.05             | -0.81             |
| IQR            | 0.04        | -0.25                          | -0.30                          | -0.08                            | 0.04                    | -0.12                         | -0.01                        | 0.27                         | -0.17            | -0.17                             | 0.08              | -0.28             |
| R <sup>2</sup> | -0.15       | 0.42                           | 0.64                           | -0.28                            | -0.30                   | 0.14                          | 0.12                         | -0.26                        | 0.27             | -0.22                             | -0.04             | 0.68              |

Table 2: Correlations between error measures (rows) and a priori and a posteriori excitation signal KPIs (columns) for APRBS 1-signal-ROMs (test set: MS15).

|                | $\bar{T}_i$ | $\overline{T_{\text{diff},i}}$ | $\overline{T_{\text{diff},j}}$ | $ \overline{T_{\text{diff},i}} $ | $\bar{T}_{\text{oven}}$ | $\text{STD}(T_{\text{oven}})$ | $\text{Cr}(T_{\text{oven}})$ | $\text{Cv}(T_{\text{oven}})$ | $\text{Cv}(T_B)$ | $\text{Cv}(T_{\text{oven}}, T_B)$ | $\text{STD}(T_A)$ | $\text{STD}(T_B)$ |
|----------------|-------------|--------------------------------|--------------------------------|----------------------------------|-------------------------|-------------------------------|------------------------------|------------------------------|------------------|-----------------------------------|-------------------|-------------------|
| RMSE           | 0.03        | 0.07                           | -0.05                          | -0.09                            | 0.04                    | 0.05                          | 0.07                         | 0.33                         | 0.12             | -0.02                             | -0.15             | -0.18             |
| MAPE           | 0.12        | 0.02                           | -0.11                          | -0.02                            | 0.14                    | 0.04                          | 0.03                         | 0.34                         | 0.13             | 0.06                              | -0.08             | -0.21             |
| MAX            | -0.21       | 0.12                           | 0.07                           | -0.21                            | -0.20                   | 0.08                          | 0.12                         | 0.23                         | 0.02             | -0.16                             | -0.24             | -0.10             |
| MEDIAN         | 0.07        | -0.56                          | -0.67                          | 0.29                             | 0.19                    | -0.03                         | -0.07                        | 0.10                         | -0.40            | 0.13                              | 0.17              | -0.53             |
| IQR            | -0.12       | 0.20                           | 0.18                           | -0.30                            | -0.17                   | 0.13                          | 0.17                         | 0.21                         | 0.16             | -0.27                             | -0.19             | 0.11              |
| R <sup>2</sup> | -0.17       | 0.34                           | 0.44                           | -0.15                            | -0.26                   | 0.07                          | 0.10                         | -0.27                        | 0.12             | -0.15                             | -0.14             | 0.41              |

---

\*Corresponding author

Email address: research@maxkann.de (Maximilian Kannapinn)

## 2. Fair test signal sets

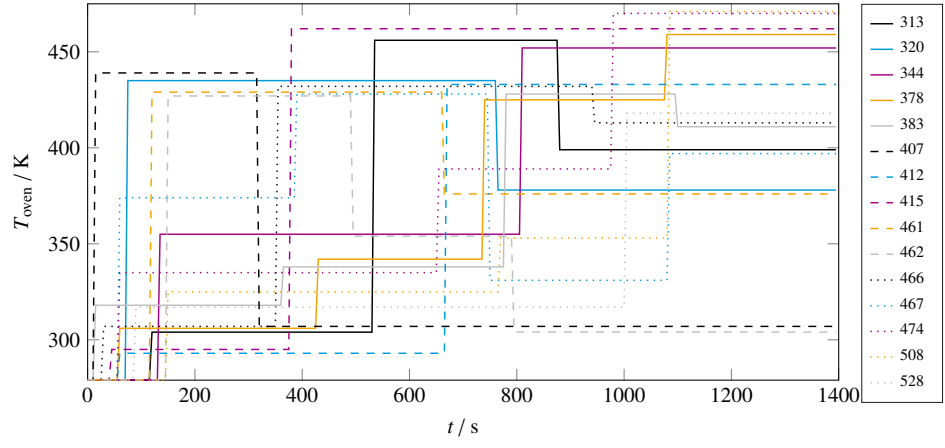

Figure 1: Fair APRBS test set AP15

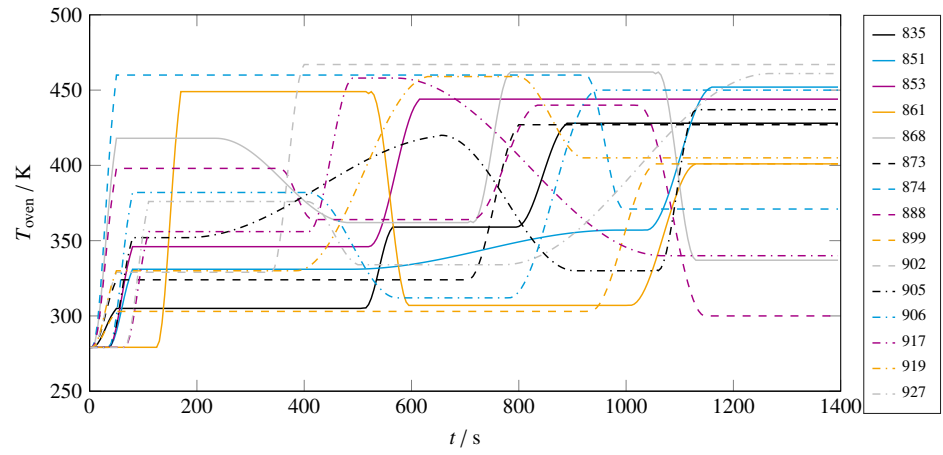

Figure 2: Fair sinAPRBS test set sinAP15

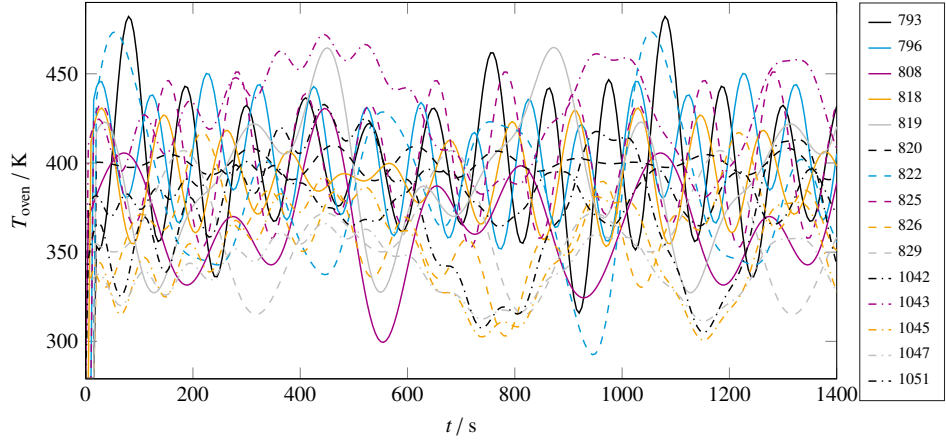

Figure 3: Fair multi-sine test set MS15

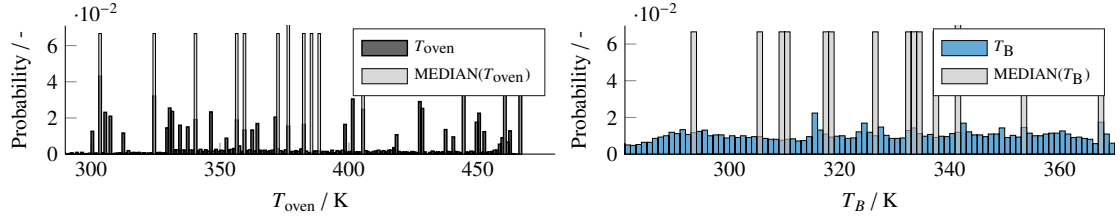

Figure 4: Fair sinAPRBS test set.

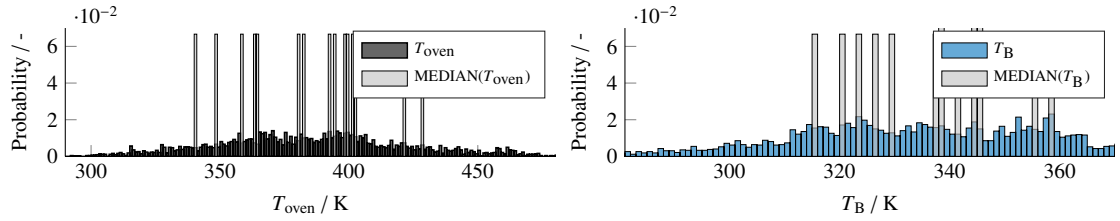

Figure 5: Fair multi-sine test set. Due to the sine character, signals with  $\text{MEDIAN}(T_{\text{oven}}) > 350$  K were chosen to obtain at least  $\text{MEDIAN}(T_B) > 310$  K.

### 3. Best training signals

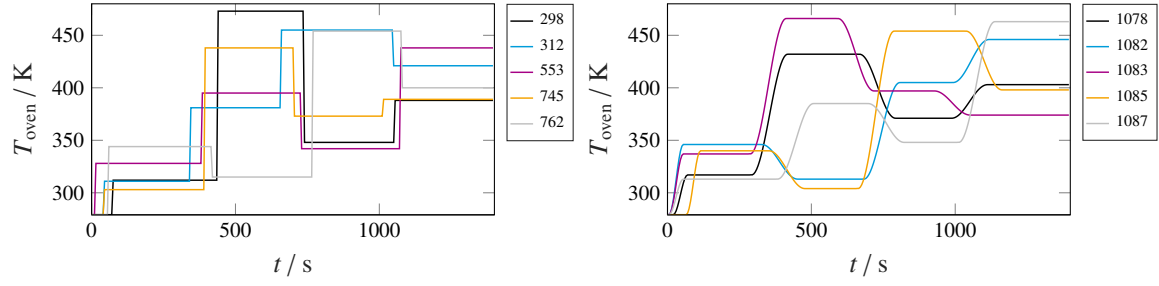

Figure 6: Best five APRBS (left) and sinAPRBS (right) training signals.

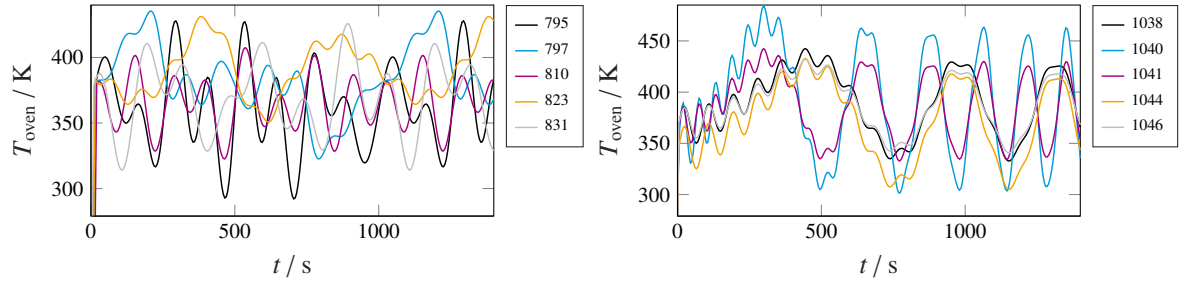

Figure 7: Best five multi-sine training signals without (left) and with (right) Schroeder phases.
